# Supplementary material for: Report of the 1st Workshop on Generative AI and Law
Source: arXiv:2311.06477 source file (2023-12-03)
Supplement: Supplementary file 2 [file 20-testimonials.tex]

\subsubsection*{Participant Testimonials}

\begin{quote}
    This was an incredibly timely workshop that focuses on one of the most important issues facing generative AI at the moment.  There are many trials testing the legitimacy of whether training AI systems on copyrighted works is fair use.  It's crucial that AI experts understand the law, and that law experts and policy makers understand AI.  This workshop is helping us build those bridges between communities.
\end{quote}

\begin{quote}
    This was one of the best workshops I've ever attended. The mix of people participating was excellent and people actually talked with one another across disciplinary boundaries. That's quite unusual. I came away with dozens of new ideas.			
\end{quote}

\begin{quote}
    It was very help to figure out the ways lawyers inadvertently confuse ML practitioners and the ways ML practitioners inadvertently confuse lawyers. Hopefully through continued collaboration we can work to clarify understanding on both sides.
\end{quote}
